# Supplementary material for: KolTa: A Physics-Informed Active Learning Framework for Formulation Discovery with Limited Data
Source: arXiv:2611.06394 source file (2026-11-06)
Supplement: Supplementary file 1 [file supplementary.tex]

% !TEX program = pdflatex
% Compile this entry point for the supplementary material.
\makeatletter
\def\input@path{{supplementary/}}
\makeatother
\input{supplementary/main.tex}
