# Supplementary material for: KolTa: A Physics-Informed Active Learning Framework for Formulation Discovery with Limited Data
Source: arXiv:2611.06394 source file (2026-11-06)
Supplement: Supplementary file 2 [file main.tex]

% !TEX program = pdflatex
\RequirePackage[T1]{fontenc}
\documentclass[journal,onecolumn]{IEEEtai}
\usepackage[utf8]{inputenc}
\usepackage{amsmath,amssymb,bm,booktabs,array,longtable,tabularx}
\usepackage{xcolor}
\usepackage{capt-of}% Caption the compact, unbroken consistency table in place.
\usepackage{cite}
\usepackage{algorithm}
\usepackage{algpseudocode}
\usepackage[hidelinks]{hyperref}
\hypersetup{pdfauthor={},pdftitle={Supplementary Material},pdfsubject={},pdfkeywords={}}
\newcommand{\method}{KolTa}
\newcommand{\R}{\mathbb{R}}
\newcommand{\Tref}{T_{\mathrm{ref}}}
\newcommand{\meany}{\widehat y}
\renewcommand{\thesection}{S\arabic{section}}
\renewcommand{\thesubsection}{\thesection.\arabic{subsection}}
\renewcommand{\thetable}{S\arabic{table}}
\renewcommand{\theequation}{S\arabic{equation}}
\renewcommand{\thepage}{S\arabic{page}}
\renewcommand{\thealgorithm}{S\arabic{algorithm}}
\renewcommand{\algorithmicrequire}{\textbf{Input:}}
\renewcommand{\algorithmicensure}{\textbf{Output:}}
\newcolumntype{Y}{>{\raggedright\arraybackslash}X}
\setlength{\LTcapwidth}{\textwidth}
% Match longtable captions to the IEEE class's regular table captions.
\makeatletter
\long\def\LT@makecaption#1#2#3{%
  \LT@mcol\LT@cols c{\hbox to\z@{\hss
    \parbox[t]\LTcapwidth{\def\@captype{table}\@makecaption{#1{#2}}{#3}}%
  \hss}}}
\makeatother
\setlength{\LTpre}{6pt}
\setlength{\LTpost}{6pt}
\begin{document}
\bstctlcite{IEEEexample:BSTcontrol}
\raggedbottom
\title{Supplementary Material\\[3pt]
\large KolTa: A Physics-Informed Active Learning Framework for Formulation Discovery with Limited Data}
\author{}
\markboth{Supplementary Material}{Supplementary Material}
\maketitle
\noindent This supplement provides implementation details and complete numerical results for the four tasks in the main manuscript: NIST, Drug, ILThermo, and DiffMix. The discovery results use the full query budget. Notation follows the main manuscript, and all reported results come from the completed runs used there. Code will be made publicly available upon acceptance.
\input{sections/model}
\input{sections/protocol}
\input{sections/results}
\input{sections/prediction}
\clearpage
\bibliographystyle{IEEEtran}
\bibliography{references}
\end{document}
