# Supplementary material for: KolTa: A Physics-Informed Active Learning Framework for Formulation Discovery with Limited Data
Source: arXiv:2611.06394 source file (2026-11-06)
Supplement: Supplementary file 3 [file model.tex]

\section{Model and Physical Constraints}\label{sec:model}
\subsection{Molecular graphs and encoder}
Each task trains its own model. The molecular encoder is shared across the components of a formulation, but its fitted weights are not shared across the four tasks.

Atoms have seven categorical inputs: atomic number, degree, formal charge, hybridization, aromaticity, total hydrogen count, and chirality. Their embedding-table sizes are 119, 9, 11, 7, 2, 9, and 4, respectively. Formal charges from $-5$ to $5$ are shifted to indices 0--10. Hybridization categories are unspecified, S, SP, SP2, SP3, SP3D, and SP3D2. Bonds have four categorical inputs: bond type, conjugation, ring membership, and stereochemistry, with embedding-table sizes 5, 2, 2, and 7. Bond types use indices 1--4 for single, double, triple, and aromatic bonds. Both directions of each bond are included. Invalid molecular inputs or unsupported categories are rejected rather than imputed.

Each categorical field has a learned 32-dimensional embedding, and the embeddings within an atom or bond are added. The encoder uses two layers of a graph isomorphism network with edge features (GINE)~\cite{hu2020}, each of width 32. The internal multilayer perceptron (MLP) has widths $32\to64\to32$ with a sigmoid linear unit (SiLU) activation. Each layer applies dropout 0.10 to its convolution output, adds this update to the input node state, and applies layer normalization.

For a molecule with $n$ atoms, the readout concatenates the mean node vector, the summed node vector divided by $\sqrt n$, and $\log(1+n)$. The resulting 65-dimensional vector passes through $65\to32\to32$, with SiLU, dropout 0.10, and final layer normalization. This produces the molecular representation $h_i\in\mathbb R^{32}$.

\subsection{Component properties and task roles}
NIST and ILThermo use one component role and append no additional component properties. ILThermo represents complete feedstocks; it does not create separate cation and anion roles. The same architecture handles its two- and three-component formulations.

Drug contains one solute and one or two positive-fraction solvents. The solute vector concatenates $h_i$ with its melting temperature, giving 33 dimensions. A solvent vector concatenates $h_i$ with its melting temperature and reference relative permittivity, giving 34 dimensions. Solvent fractions sum to one within the solvent mixture. The saturated solute mole fraction is the prediction target and is not provided as an input.

Drug properties are standardized separately within each role using the unique compounds in the fitting formulations. Repeated temperature records and bootstrap multiplicities do not duplicate compounds when fitting these statistics. Validation formulations do not contribute to fitting the scaler. For a property with mean $\mu$ and population standard deviation $\sigma$, the transformation is $(a-\mu)/d$, where
\begin{equation}
 f=0.01\max(|\mu|,1),\qquad
 d=\begin{cases}
  \max(\sigma,f), & \sigma>10^{-12},\\
  \max(1,f), & \text{otherwise.}
 \end{cases}
\end{equation}
Values are not clipped after transformation. Missing, nonfinite, or nonpositive required properties are rejected; there is no missing-value imputation or missingness indicator.

DiffMix has one whole-salt component and one to three positive-fraction solvent components. Salt and solvent roles use a two-element one-hot encoding. Its fractions are defined over whole-salt formula units and solvent molecules. If the source gives equal cation and anion amounts $q$ and solvent amounts $a_j$, the single whole-salt fraction is $q/(q+\sum_j a_j)$, and solvent fractions are $a_j/(q+\sum_j a_j)$. The salt amount is counted once.

\subsection{Three-stage networks}
Table~\ref{tab:slayers} specifies the networks used after component encoding. A width list gives the input, hidden, and output dimensions. Component and message MLPs use SiLU and dropout 0.10; message outputs also use layer normalization. The interaction projections and interaction scalar readout have no bias. Only the permitted directed pairs of distinct components generate messages.

\begin{table}[htbp]
\centering\small
\caption{Network dimensions by task. Drug adds auxiliary properties before these networks. $H(F)$ supplies both the temperature and physics coefficient heads.}
\label{tab:slayers}
\renewcommand{\arraystretch}{1.15}
\begin{tabularx}{\textwidth}{@{}lYYY@{}}
\toprule
Module & NIST / ILThermo & Drug & DiffMix\\
\midrule
Base contribution $g_C$ & $32\to16\to1$ & $35\to16\to1$ & $34\to16\to1$\\
Pair message $f$ & $66\to32\to16$ & $68\to32\to16$ & $66\to32\to16$ per type\\
Message projection $W$ & $16\to32$ & $16\to32$ & $16\to32$ per type\\
Receiver output $O$ & $32\to32$ & $32\to32$ & $32\to32$ per role\\
Interaction readout $g_I$ & $32\to16\to1$ & $32\to16\to1$ & $32\to16\to1$\\
Context dimension $H(F)$ & 64 & 65 & 64\\
Temperature network $q_\phi$ & $65\to16\to1$ & $66\to16\to1$ & $65\to16\to1$\\
Physics coefficient head & $64\to1$ & $65\to1$ & $64\to2$\\
\bottomrule
\end{tabularx}
\end{table}

For viscosity, all components enter the base and interaction readouts with mole-fraction weights. Each pair message receives the two 32-dimensional component vectors and both fractions. Drug uses only solvent-to-solute messages: the pair input has 33 solute features, 34 solvent features, and one solvent fraction. Its base head receives the 33 solute features and the two-element role encoding. Only the solute enters the readout, with weight one. DiffMix uses three separate message functions: salt$\leftarrow$solvent, solvent$\leftarrow$salt, and solvent$\leftarrow$solvent. All components enter its mole-fraction-weighted readouts.

For every task, a message is multiplied by the sender fraction before aggregation. Incoming messages are grouped by sender role, projected by $W$, added, passed through SiLU, and mapped by $O$. The interaction readout $g_I$ uses SiLU with no dropout. The context concatenates the weighted component representation with the 32-dimensional interaction vector. The temperature network $q_\phi$ uses SiLU and no dropout. Both evaluations in $q_\phi(H(F),t)-q_\phi(H(F),0)$ reuse the same static representation, so the anchored difference is zero at $t=0$, including during training.

\subsection{Temperature coordinates and coefficient maps}
Temperatures are in K and $t=(T-T_{\rm ref})/s_T$. The reference and scale are $(298.15,10)$ for NIST, $(303.15,50)$ for Drug, $(313.15,10)$ for ILThermo, and $(268.15,25)$ for DiffMix. Selection uses $t^*=0$ for the three measured tasks and $t^*=1$ for DiffMix.

For viscosity and solubility, a linear scalar output $a(H)$ is rescaled as
\begin{equation}
 \theta(F)=\frac{T_{\rm ref}^2}{s_T}a(H(F)).
\end{equation}
The coefficient is unrestricted in sign. The corresponding derivatives of the logarithmic target are $-\theta/T^2$ for viscosity~\cite{chemixhub} and $+\theta/T^2$ for solubility~\cite{moreno2022solubility}. For DiffMix, two linear outputs $a(H)$ and $b(H)$ give
\begin{equation}
 \beta(F)=\frac{(268.15-233.15/2)^2}{25}\operatorname{softplus}(a(H)),
 \qquad T_0(F)=233.15\operatorname{sigmoid}(b(H)).
\end{equation}
For DiffMix, the two-output coefficient head is initialized with zero weights and biases $(\log(\exp(0.1)-1),0)$, giving $\beta\approx91.900$ and $T_0=116.575$~K. The VFT derivative is $\beta/(T-T_0)^2$~\cite{diffmix}. The upper bound on $T_0$ is 10 K below the lowest collocation temperature. All coefficients depend on the formulation but remain constant while temperature varies. These are fitted coefficients of a soft constraint, rather than independently measured physical constants.

The physics loss follows the residual-penalty approach of physics-informed learning~\cite{raissi} and evaluates the residual at five fixed temperatures:
\begin{itemize}
\item NIST and Drug: $[293.15,\ 298.0661495891,\ 303.15,\ 308.0688706799,\ 313.15]$ K. The two interior off-center points are harmonic means of each adjacent endpoint and 303.15 K.
\item ILThermo: $[303.15,\ 307.9142621405,\ 312.8306642184,\ 317.9066120396,\ 323.15]$ K, equally spaced in inverse temperature.
\item DiffMix: $[243.15,\ 255.65,\ 268.15,\ 280.65,\ 293.15]$ K, equally spaced in temperature.
\end{itemize}
The fixed collocation ranges do not restrict the measured records used in the data loss. Evaluating the residual requires no measured target at a collocation temperature.
