# Supplementary material for: KolTa: A Physics-Informed Active Learning Framework for Formulation Discovery with Limited Data
Source: arXiv:2611.06394 source file (2026-11-06)
Supplement: Supplementary file 4 [file prediction.tex]

\section{Prediction Error on the Locked Sets}\label{sec:prediction}
The locked sets contain 3,894 NIST, 524 Drug, 486 ILThermo, and 368 DiffMix formulations. They are excluded from training, hyperparameter selection, calibration, and acquisition. Table~\ref{tab:smae} reports the MAE of the final ensemble or GP prediction at the target temperature, after the initial set and all ten acquisition rounds. The resulting training budgets are 1,000, 1,100, 450, and 500 formulations, respectively.

Errors are measured in the same base-10 logarithmic units used for training: viscosity in cP, saturated solute mole fraction, and conductivity in S/cm before taking the logarithm. Each locked formulation contributes one target-temperature prediction. The table includes all model--acquisition combinations in the main comparison; Random has no fitted predictor in this analysis.

Each final model was trained on the formulations selected by its own strategy, so this comparison includes the effects of both the predictor and the selected data.
\input{tables/mae}
