# Supplementary material for: KolTa: A Physics-Informed Active Learning Framework for Formulation Discovery with Limited Data
Source: arXiv:2611.06394 source file (2026-11-06)
Supplement: Supplementary file 5 [file protocol.tex]

\section{Data, Training, and Comparator Settings}\label{sec:protocol}
\subsection{Data preparation and query allocation}
All temperature records belonging to the same formulation remain together when splitting data. A formulation is identified by its components and composition, with temperature stored as a condition. Candidates must have a target-temperature record for evaluation. Discovery-pool membership and the locked split are established before acquisition. The locked set never contributes to fitting or model selection. The NIST, Drug, and ILThermo measurement datasets are distributed by CheMixHub~\cite{chemixhub}.

NIST~\cite{kazakov2012source} retains 19,469 formulations and 50,429 condition records at 101 kPa. The 20\% locked split uses seed 20260923 and rounds its size upward. Four sources are excluded before aggregation for all methods. Source \texttt{ref11189} has unresolved discrepancies in numerical scale within the source. Source \texttt{ref64946} has an unresolved numerical-scale conflict with other sources. Source \texttt{ref13743} contains conflicting repeated measurements at the same conditions. Source \texttt{ref126833} is excluded because its measurement conditions remain unresolved. Measurements from other sources for the same formulation are retained. Repeated retained measurements at an identical formulation, temperature, and pressure are aggregated in logarithmic viscosity units.

ILThermo~\cite{dong2007ilthermo} retains 2,426 formulations and 17,072 condition records at 100 kPa. The 20\% locked split uses seed 20261015 and rounds upward. Preparation removes duplicates within a source before averaging retained logarithmic viscosity values across sources. DiffMix~\cite{diffmix} retains 1,839 formulations and 11,022 simulated condition records. Its locked split uses seed 20261016 and the same upward rounding; identical condition values are deduplicated.

For Drug~\cite{bao2024solubility}, preparation starts from 3,019 formulations with target-temperature records. We remove 62 formulations belonging to two drugs with missing melting-point data. We then retain drug groups with at least twelve formulations in the discovery pool, removing another 274 formulations. Each retained formulation keeps its discovery-pool or locked-set assignment. This gives 86 drug groups, 2,683 formulations, and 23,688 condition records. Nine exact duplicate records and two conflicting condition measurements are removed during preparation; no target-temperature conflicts remain. The retained records span 263.15--353.15 K, including records outside the collocation range.

Drug initializes 300 formulations using a balanced allocation across drugs. At each allocation step, a nonexhausted group with the smallest allocated count is selected, with seeded tie-breaking; initialization then draws an unused formulation randomly within that group. Later query slots follow the same minimum-count rule, with the group sequence fixed before access to unknown targets. Each acquisition rule selects within the scheduled group. The schedule uses base seed 2026101401 and repeat indices 0, 1, and 2. Model fitting and calibration pool all currently labeled formulations rather than fitting one model per drug.

Table~\ref{tab:stasks} summarizes the pools, targets, and budgets. By the end of a run, 6\% of the NIST pool is labeled, compared with 51\% of the Drug pool. The tasks have 74 to 779 targets. The initial labeled set contains 4 to 22 of them, and these are excluded from active recall. On Drug, 77 to 82 of the 86 drugs keep at least one target after initialization. NIST formulations have a median of two temperature records, and Drug formulations nine.
\input{tables/taskstats}

\subsection{Model selection and ensemble refitting}
Table~\ref{tab:straining} gives the shared neural search settings. Model selection uses mean absolute error (MAE) at the target temperature. Each training batch contains sampled formulations and all their temperature records. Mean squared error (MSE) is first averaged within each formulation, then across the sampled formulations. If a formulation is drawn more than once in a bootstrap sample, its loss is counted once per draw. The physics loss uses the same formulation and bootstrap weighting.

\begin{table}[htbp]
\centering\small
\caption{Neural training and selection settings. \method{} and its variants A1 and A2 search twelve combinations; the neural comparators search four. XGBoost and GP use the separate procedures below.}
\label{tab:straining}
\renewcommand{\arraystretch}{1.12}
\begin{tabularx}{\textwidth}{@{}lY@{}}
\toprule
Setting & Value\\
\midrule
Bootstrap ensemble size & 5\\
Outer out-of-fold (OOF) folds & 5, grouped by formulation, for calibrated acquisition; omitted for Greedy\\
Inner validation fraction & 0.20 of fitting formulations\\
Learning rate & $\{3\times10^{-4},10^{-3}\}$\\
Weight decay & $\{0,10^{-4}\}$\\
Physics-loss weight $\lambda$ & $\{0.01,0.1,1\}$ for \method{}, A1, and A2\\
Maximum epochs & 500\\
Early-stopping patience & 50 epochs without a validation-MAE improvement exceeding $10^{-8}$\\
Batch size & 16 formulation draws\\
Hyperparameter selection & Target-temperature validation MAE of one temporary member per setting\\
Full-model optimizer & Adam~\cite{kingma2015adam}\\
\bottomrule
\end{tabularx}
\end{table}

For a fitting set of size $n$, a seeded permutation of its sorted formulation IDs selects $\min(n-1,\max(1,\lceil0.2n\rceil))$ validation formulations. This is a formulation split, including for Drug, rather than a leave-one-drug-out split. All grid settings use a common initialization/order seed. Ties in the best validation MAE are resolved lexicographically by learning rate, weight decay, and physics weight.

After selection, each ensemble member draws $n$ formulations with replacement from the entire fitting set. A freshly initialized model is trained for the epoch count attaining the best inner-validation MAE for the selected setting, without a validation holdout or further early stopping. Each member's feature scaler is fitted only on the formulations in its bootstrap sample. The full predictor trains on the prepared logarithmic target without a further target z-score transform. Its scalar bias starts at the bootstrap-weighted mean of target-temperature fitting labels.

\subsection{OOF predictions and acquisition calibration}
For Physics-Residual-Calibrated Upper Confidence Bound (PRC-UCB) and its $u$-only variant A1, we obtain grouped out-of-fold (OOF) predictions. Outer folds depend only on formulation identifiers (IDs) and a seed. For each ID, we hash the string \texttt{group-oof::\allowbreak seed::\allowbreak ID} with SHA-256. We sort the IDs by these hashes and assign them cyclically to five folds. Each held-out fold is excluded from feature scaling, inner selection, and ensemble fitting; the remaining four folds undergo the complete selection and refitting procedure above. This gives one target-temperature OOF prediction per labeled formulation.

The uncertainty signal $u$ is the sample standard deviation of the five predictions. The physics signal $v$ is the mean absolute residual of the five members, evaluated at the target temperature. The calibration response is $s(y-\tilde\mu)$, with $s=+1$ for NIST, Drug, and DiffMix and $s=-1$ for ILThermo. Drug uses one global coefficient pair with equal weight per labeled formulation.

We fit nonnegative coefficients without an intercept by minimizing the pinball loss with $\tau=0.8$~\cite{koenker}. Each nonzero signal column is divided by its root mean square (RMS); the response is also scaled by its maximum absolute value for the numerical solve. The HiGHS solver~\cite{huangfu2018highs}, accessed through SciPy~\cite{virtanen2020scipy}, solves the linear program with primal and dual feasibility tolerances of $10^{-9}$. Among solutions attaining the minimum loss to numerical tolerance, a second step selects the smallest coefficient norm in the scaled coordinates. Its base loss tolerance is $10^{-9}\max(1,|L_{\min}|)$ in the scaled problem. The implementation uses up to 256 cutting-plane steps, with sequential least-squares programming (SLSQP)~\cite{kraft1988slsqp} tolerance $10^{-13}$ and at most 200 iterations per step. The coefficients are then converted back to the original signal units.

A column that is identically zero receives coefficient zero. If all signals or all signed errors are zero, the fitted margin is zero. A1 refits the calibration with the residual column omitted; it does not simply retain the full method's fitted $u$ coefficient.

The comparators' upper confidence bound (UCB) rule instead uses $\gamma=\operatorname{RMS}(e)/\operatorname{RMS}(u)$, clipped to $[0.25,4]$. It falls back to $\gamma=1$ with fewer than ten positive-weight OOF rows or $\operatorname{RMS}(u)\le10^{-6}$. Greedy selection uses each predictor's own mean and does not need OOF calibration. After the final acquisition batch, the model is refitted for evaluation.

\subsection{One acquisition round}
Algorithm~\ref{alg:round} summarizes one round of \method{} with the settings above. A1 fits $c_u$ alone in line~7. The greedy variant A2 omits lines~1--7 and ranks candidates by $s\,\mu(F)$.

\begin{algorithm}[htbp]
\caption{One acquisition round of \method{}}\label{alg:round}
\begin{algorithmic}[1]
\Require Labeled set $\mathcal L_\ell$ with all measured records, unlabeled set $\mathcal U_\ell$, batch size $b$, target temperature $T^*$, and objective sign $s$
\Ensure Next batch $\mathcal Q_\ell$ and labeled set $\mathcal L_{\ell+1}$
\State Split $\mathcal L_\ell$ into five folds of formulations
\For{$k=1,\dots,5$}
\State Select the learning rate, weight decay, and $\lambda$ on an inner validation split of the other four folds
\State Train five bootstrap members on the other four folds with the selected setting
\State For each $F$ in fold $k$, compute $\tilde\mu(F)$, $\tilde u(F)$, and $\tilde v(F)$ at $T^*$, and $e(F)=s\bigl(y(F,T^*)-\tilde\mu(F)\bigr)$
\EndFor
\State Fit $(c_u,c_v)\ge0$ by the pinball loss at $\tau=0.8$ on RMS-scaled signals, keeping the minimum-norm solution
\State Select the setting on an inner validation split of $\mathcal L_\ell$, and train five bootstrap members on $\mathcal L_\ell$
\State For each $F\in\mathcal U_\ell$, compute $\mu(F)$, $u(F)$, and $v(F)$ at $T^*$, and $\alpha(F)=s\,\mu(F)+c_u u(F)+c_v v(F)$
\State $\mathcal Q_\ell\gets$ the $b$ candidates with the highest $\alpha(F)$; on Drug, the highest in each scheduled drug slot
\State Query $\mathcal Q_\ell$, return all records $\mathcal O_F$ of each $F\in\mathcal Q_\ell$, and set $\mathcal L_{\ell+1}\gets\mathcal L_\ell\cup\mathcal Q_\ell$
\end{algorithmic}
\end{algorithm}

\subsection{Comparator implementations}
\textbf{Gaussian process (GP).} The exact GP~\cite{rasmussen2006gaussian} uses BoTorch 0.17.1~\cite{balandat2020botorch} \texttt{SingleTaskGP}, a squared-exponential kernel with automatic relevance determination, and a Gaussian likelihood. Inputs contain 200 composition-weighted, histogram-normalized RDKit descriptors~\cite{rdkit,kelley_descriptastorus} plus temperature for NIST, ILThermo, and DiffMix. Drug concatenates 200 solvent-mixture descriptors, 200 solute descriptors, the solute melting temperature, mixture-weighted solvent melting temperature and relative permittivity, and temperature (404 dimensions). The fixed external descriptor transform is \texttt{rdkit2dhistogramnormalized}; it fits no candidate or target values. Temperature enters in K. Input min/max normalization and output standardization are fitted only on the training records. A near-constant input range below $10^{-8}$ is replaced by one.

The GP uses one likelihood row per measured condition and fits the exact marginal likelihood in double precision using L-BFGS-B~\cite{byrd1995lbfgsb}, capped at 200 iterations. It uses neither bootstrap ensembles nor OOF calibration. Finite optimizer results with status \texttt{STOPPED} are accepted; failures or nonfinite results are rejected. Thus the specified fitting budget does not require optimizer convergence at every round.

Expected improvement (EI)~\cite{jones} is evaluated in logarithmic form~\cite{ament2023unexpected}. GP-EI constructs batches sequentially with this score and a Kriging believer~\cite{ginsbourger2010kriging}. The incumbent is fixed to the best observed target-temperature utility at the beginning of the real round. After each selection, posterior-mean fantasy values are added for all recorded temperatures of that formulation, without refitting kernel hyperparameters within the batch. GP-Greedy ranks candidates by the posterior mean. Posterior uncertainty is latent uncertainty, with observation noise excluded.

\textbf{XGBoost.} XGBoost~\cite{chen2016xgboost} uses five bootstrap members with squared-error boosting, maximum tree depth 3, learning rate 0.03, minimum child weight 3, $L_2$ regularization 5, and $L_1$ regularization 0.05. The histogram tree method runs on the CPU with four threads. Validation MAE selects the number of boosting rounds, with a cap of 300 and patience 50; final members replay the selected count. Each record is weighted by its formulation's bootstrap multiplicity divided by that formulation's number of records. XGBoost uses the fixed \texttt{RDKit2DNormalized} cumulative-distribution transform~\cite{kelley_descriptastorus} followed by fitting-support standardization, with task-normalized temperature. Inputs have 201 dimensions for NIST and DiffMix, 404 for Drug, and 205 for ILThermo. ILThermo appends four mole-fraction-weighted missing-charge indicators to the 200 descriptors before adding temperature. These indicators correspond to maximum/minimum signed and absolute partial-charge descriptors. Missing charge values are zero-filled, while unexpected missing descriptors are rejected. The four indicators are not standardized. The neural learning-rate/weight-decay grid is not searched for these trees.

\textbf{MolSets.} The adapted MolSets model~\cite{molsets} uses three graph-convolution layers of width 16, a 32-dimensional embedding with tanh, and an attention width of 16. It retains column-softmax attention and composition-weighted set aggregation. Its 14 atom features comprise the original 13 features and a missing-electronegativity flag; missing electronegativity is zero-filled with this flag. Molecular weights enter the mixture representation. Public mole fractions are converted to mass fractions for aggregation.

Drug uses a separate solute encoder and a solvent-only mixture representation. Its context contains normalized temperature and the three auxiliary properties; the other tasks use temperature context only. MolSets uses AdamW~\cite{loshchilov2019adamw}. For each member, the target mean and population standard deviation are fitted from all temperature records of the distinct formulations in its bootstrap sample, without repeating records when a formulation is drawn more than once. A standard deviation below $10^{-8}$ is replaced by one. Training uses standardized squared errors with formulation/bootstrapping weights, while validation MAE is calculated in the original logarithmic target units.

\textbf{SolvGNN.} The adapted SolvGNN model~\cite{solvgnn} uses hidden width 128, two local graph-convolution layers, one component-level message update using a gated recurrent unit (GRU)~\cite{cho2014gru}, and an edge-network hidden width of 32. Its atom representation extends the 74 canonical features with Ne and Kr. Molecular bonds are bidirectional, with one self-loop per atom. Component-edge hydrogen-bond features use RDKit donor/acceptor counts.

NIST, ILThermo, and DiffMix use mole-fraction-weighted component readout and temperature context. Drug reads the updated solute node, uses solvent fractions, and fills the unknown solute fraction with zero alongside an explicit unknown-fraction indicator. Its context contains the same four quantities as MolSets. SolvGNN uses Adam~\cite{kingma2015adam} and the prepared-target MSE, with the shared formulation weighting, neural grid, and target-temperature validation procedure.

\subsection{Software environment}
The saved run manifests record Python 3.12.3 or 3.12.13 and RDKit 2026.03.5. For acquisition runs, \method{} uses PyTorch 2.5.1+cu124 on NIST and 2.13.0 on Drug, ILThermo, and DiffMix; A1 and A2 also use 2.13.0. The graph and GP comparators use PyTorch 2.8.0+cu128, 2.12.1+cu130, or 2.13.0, depending on the task and strategy. Recorded SciPy versions are 1.18.0 and 1.18.1. The accompanying \texttt{software\_versions.csv} gives the recorded versions for each reported task--strategy combination across seeds 0, 1, and 2.
