# Supplementary material for: KolTa: A Physics-Informed Active Learning Framework for Formulation Discovery with Limited Data
Source: arXiv:2611.06394 source file (2026-11-06)
Supplement: Supplementary file 6 [file results.tex]

\section{Detailed Discovery Results}\label{sec:results}
\subsection{Full-budget AULC and query counts}
Area under the learning curve (AULC) is calculated from active recall after each batch, using the trapezoidal rule and dividing by the total number of new queries. The budgets are 800 for NIST, 800 for Drug, 300 for ILThermo, and 400 for DiffMix. Targets found in the initial labeled set are excluded from both the numerator and denominator of active recall. Drug averages recall equally across drug groups with targets remaining after initialization.

Table~\ref{tab:saulc} gives the individual runs behind the main manuscript's summary table. Each model--acquisition combination in the main comparison is reported separately. The three measured tasks (NIST, Drug, and ILThermo) evaluate all nine strategies; the simulated DiffMix task evaluates six strategies, omitting MolSets-Greedy, SolvGNN-Greedy, and GP-Greedy. Random is evaluated using three saved replays on each task, with the same initial sets and query budgets as the model-based strategies. We report each replay's AULC, their mean, and sample standard deviation. Drug replays follow the balanced group schedule.
\input{tables/aulc}
MolSets-UCB's low DiffMix AULC reflects slow early recovery: all three runs complete the full budget and recover 85.7--92.3\% of the remaining targets, but only 5.7--30.8\% after 160 new queries. The saved batches follow the UCB scores; in eight of the twelve batches from the first four rounds across the three runs, the selected 40 candidates have no overlap with the 40 highest predicted means in the same saved candidate pool. These rankings show the exploration margin redirecting early queries.

Table~\ref{tab:squeries} gives the query counts used to calculate the main manuscript's $q_{30}$ and $q_{80}$ summaries. The median is taken only over runs that reach the requested recall; a missing value is not replaced by the budget.
\input{tables/queries}

\subsection{Paired statistical comparisons}
For each comparator, we subtract its full-budget AULC from that of \method{} at the same task and seed. There are twelve pairs when a strategy was run on all four tasks and nine for the three greedy strategies that were not run on DiffMix. Positive differences favor \method{}. Table~\ref{tab:stests} provides the complete comparisons summarized in the main manuscript.

The one-sided sign test uses the number of positive nonzero differences under a binomial null with probability $1/2$. The one-sided Wilcoxon signed-rank test~\cite{wilcoxon1945} ranks the absolute nonzero differences and obtains the tail probability by enumerating all sign assignments. The implementation excludes zero differences and uses average ranks for tied magnitudes; neither occurs in these eight comparisons. Holm adjustment~\cite{holm1979} is applied separately to the eight sign-test $p$ values and the eight Wilcoxon $p$ values. The main manuscript reports support when both adjusted values are below 0.05.

\input{tables/tests}

\subsection{Predictor and acquisition analyses}
\textbf{Predictor and acquisition variants.} Table~\ref{tab:sablations} gives the two-task variant results. A1 uses the full predictor and physics loss but fits the acquisition margin using ensemble disagreement $u$ alone ($c_v=0$). A2 uses the full predictor and physics loss with greedy acquisition. Its results and the greedy comparator results in Table~\ref{tab:saulc} provide the predictor comparison under a common acquisition rule. Each variant selects its own formulations and retrains on the records it acquires, so these comparisons include both selection and subsequent learning.

In these descriptive comparisons, adding the residual to the calibrated margin improves AULC in five of six runs. \method{} achieves higher AULC than greedy A2 in all three Drug runs and one of three ILThermo runs. Its sample standard deviation is lower than A2's on both tasks.
\input{tables/ablation}

\textbf{Cross-task consistency analysis.} To complement the task-specific comparisons, we summarize cross-task consistency using per-run ranks and gaps to the best mean AULC. We rank the nine model-based strategies within each task and seed using the AULCs reported in Table~\ref{tab:saulc}. For each task, a strategy's gap is the highest mean AULC among these nine strategies minus its own mean AULC. We take the largest gap across NIST, Drug, and ILThermo, where all nine strategies were evaluated. Table~\ref{tab:sconsistency}(a) reports the per-run ranks, the number of runs in the top three, and each strategy's maximum gap.

For the acquisition variants, the reference on each task is the highest mean AULC among PRC-UCB, A1, and A2. We take the larger gap across Drug and ILThermo. Table~\ref{tab:sconsistency}(b) gives the task means and maximum gaps. Rankings and gaps use unrounded values. The accompanying numerical files provide the task-level gaps and all per-run ranks.
\input{tables/consistency}

\subsection{Calibrated margin coefficients}
Table~\ref{tab:scalib} summarizes the coefficients fitted in the 30 acquisition rounds of each task. In the RMS-scaled coordinates, each coefficient multiplies a signal divided by its root mean square over the labeled formulations, so the two coefficients can be compared. The disagreement coefficient $c_u$ is positive in every round. The residual coefficient $c_v$ is positive in 115 of the 120 rounds, so the fitted margin uses the physics residual on all four tasks. On every task, the median scaled residual coefficient is smaller than the median scaled disagreement coefficient, with the weights refitted each round to the out-of-fold signed errors on each task.
\input{tables/calibration}
