# Supplementary material for: KolTa: A Physics-Informed Active Learning Framework for Formulation Discovery with Limited Data
Source: arXiv:2611.06394 source file (2026-11-06)
Supplement: Supplementary file 7 [file ablation.tex]

{\small\setlength{\tabcolsep}{3.2pt}\renewcommand{\arraystretch}{1.12}
\begin{longtable}{@{}p{0.28\textwidth}rrrrrrrr@{}}
\caption{Full-budget results for \method{} and its acquisition variants. AULC uses the same budget as the main comparison. Each variant selects its own formulations and is retrained along its own trajectory. All reported runs reach 80\% recall.}\label{tab:sablations}\\
\toprule
& \multicolumn{5}{c}{AULC} & \multicolumn{3}{c}{$q_{80}$}\\
\cmidrule(lr){2-6}\cmidrule(l){7-9}
Variant & Seed 0 & Seed 1 & Seed 2 & Mean & SD & Seed 0 & Seed 1 & Seed 2 \\
\midrule
\endfirsthead
\multicolumn{9}{c}{\tablename~\thetable\ (continued)}\\
\toprule
& \multicolumn{5}{c}{AULC} & \multicolumn{3}{c}{$q_{80}$}\\
\cmidrule(lr){2-6}\cmidrule(l){7-9}
Variant & Seed 0 & Seed 1 & Seed 2 & Mean & SD & Seed 0 & Seed 1 & Seed 2 \\
\midrule
\endhead
\midrule
\multicolumn{9}{r}{Continued on next page}\\
\endfoot
\bottomrule
\endlastfoot
\multicolumn{9}{l}{\textbf{Drug}}\\
\method{} (ours) & 0.7444 & 0.7485 & 0.7222 & 0.7384 & 0.0141 & 310.3 & 348.0 & 353.1 \\
A1: margin with $u$ only & 0.7264 & 0.7263 & 0.7356 & 0.7294 & 0.0053 & 341.6 & 377.7 & 360.2 \\
A2: greedy & 0.6943 & 0.7304 & 0.7112 & 0.7120 & 0.0181 & 414.2 & 355.1 & 382.6 \\
\multicolumn{9}{l}{\textbf{ILThermo}}\\
\method{} (ours) & 0.7351 & 0.7333 & 0.7753 & 0.7479 & 0.0237 & 112.0 & 114.5 & 103.2 \\
A1: margin with $u$ only & 0.7298 & 0.7300 & 0.7478 & 0.7359 & 0.0103 & 114.0 & 115.4 & 121.7 \\
A2: greedy & 0.7340 & 0.7478 & 0.8071 & 0.7630 & 0.0389 & 114.3 & 107.6 & 92.2 \\
\end{longtable}
}
