# Supplementary material for: KolTa: A Physics-Informed Active Learning Framework for Formulation Discovery with Limited Data
Source: arXiv:2611.06394 source file (2026-11-06)
Supplement: Supplementary file 8 [file aulc.tex]

{\small\renewcommand{\arraystretch}{1.12}
\begin{longtable}{@{}lrrrrr@{}}
\caption{Full-budget AULC for every reported strategy. Higher is better. SD is the sample standard deviation across three runs. Random uses three replays on every task.}\label{tab:saulc}\\
\toprule
Strategy & Seed 0 & Seed 1 & Seed 2 & Mean & SD \\
\midrule
\endfirsthead
\multicolumn{6}{c}{\tablename~\thetable\ (continued)}\\
\toprule
Strategy & Seed 0 & Seed 1 & Seed 2 & Mean & SD \\
\midrule
\endhead
\midrule
\multicolumn{6}{r}{Continued on next page}\\
\endfoot
\bottomrule
\endlastfoot
\multicolumn{6}{l}{\textbf{NIST}}\\
\method{} (ours) & 0.4437 & 0.4366 & 0.4512 & 0.4439 & 0.0073 \\
MolSets-UCB & 0.3008 & 0.3236 & 0.3015 & 0.3086 & 0.0130 \\
MolSets-Greedy & 0.4132 & 0.3913 & 0.4055 & 0.4033 & 0.0111 \\
SolvGNN-UCB & 0.3769 & 0.3710 & 0.3917 & 0.3799 & 0.0107 \\
SolvGNN-Greedy & 0.4283 & 0.4529 & 0.4394 & 0.4402 & 0.0123 \\
GP-EI & 0.1335 & 0.1205 & 0.1119 & 0.1220 & 0.0109 \\
GP-Greedy & 0.4739 & 0.4860 & 0.4680 & 0.4760 & 0.0092 \\
XGBoost-UCB & 0.4073 & 0.3932 & 0.3953 & 0.3986 & 0.0076 \\
XGBoost-Greedy & 0.4034 & 0.4190 & 0.3816 & 0.4013 & 0.0188 \\
Random & 0.0296 & 0.0242 & 0.0291 & 0.0276 & 0.0030 \\
\addlinespace[4pt]
\multicolumn{6}{l}{\textbf{Drug}}\\
\method{} (ours) & 0.7444 & 0.7485 & 0.7222 & 0.7384 & 0.0141 \\
MolSets-UCB & 0.6578 & 0.6244 & 0.6692 & 0.6505 & 0.0233 \\
MolSets-Greedy & 0.6528 & 0.6722 & 0.6520 & 0.6590 & 0.0115 \\
SolvGNN-UCB & 0.6847 & 0.6662 & 0.6963 & 0.6824 & 0.0152 \\
SolvGNN-Greedy & 0.6704 & 0.6855 & 0.6903 & 0.6821 & 0.0104 \\
GP-EI & 0.6399 & 0.6515 & 0.7042 & 0.6652 & 0.0343 \\
GP-Greedy & 0.6608 & 0.6617 & 0.6351 & 0.6526 & 0.0151 \\
XGBoost-UCB & 0.6140 & 0.5806 & 0.5746 & 0.5897 & 0.0212 \\
XGBoost-Greedy & 0.6039 & 0.6661 & 0.6201 & 0.6300 & 0.0323 \\
Random & 0.2408 & 0.1845 & 0.2598 & 0.2284 & 0.0391 \\
\addlinespace[4pt]
\multicolumn{6}{l}{\textbf{ILThermo}}\\
\method{} (ours) & 0.7351 & 0.7333 & 0.7753 & 0.7479 & 0.0237 \\
MolSets-UCB & 0.7043 & 0.7044 & 0.7192 & 0.7093 & 0.0086 \\
MolSets-Greedy & 0.6441 & 0.6944 & 0.7346 & 0.6911 & 0.0453 \\
SolvGNN-UCB & 0.7053 & 0.6411 & 0.7148 & 0.6871 & 0.0401 \\
SolvGNN-Greedy & 0.7330 & 0.6822 & 0.7445 & 0.7199 & 0.0331 \\
GP-EI & 0.2686 & 0.1550 & 0.2137 & 0.2125 & 0.0568 \\
GP-Greedy & 0.6585 & 0.7822 & 0.7626 & 0.7345 & 0.0665 \\
XGBoost-UCB & 0.6516 & 0.7294 & 0.6791 & 0.6867 & 0.0395 \\
XGBoost-Greedy & 0.6553 & 0.6561 & 0.7055 & 0.6723 & 0.0287 \\
Random & 0.0931 & 0.0378 & 0.1121 & 0.0810 & 0.0386 \\
\addlinespace[4pt]
\multicolumn{6}{l}{\textbf{DiffMix}}\\
\method{} (ours) & 0.8500 & 0.8069 & 0.8500 & 0.8356 & 0.0249 \\
MolSets-UCB & 0.2957 & 0.3892 & 0.2921 & 0.3257 & 0.0551 \\
SolvGNN-UCB & 0.7929 & 0.7977 & 0.8543 & 0.8149 & 0.0342 \\
GP-EI & 0.6571 & 0.5877 & 0.6314 & 0.6254 & 0.0351 \\
XGBoost-UCB & 0.7814 & 0.7669 & 0.8214 & 0.7899 & 0.0282 \\
XGBoost-Greedy & 0.8400 & 0.8531 & 0.8207 & 0.8379 & 0.0163 \\
Random & 0.1129 & 0.1562 & 0.1279 & 0.1323 & 0.0220 \\
\end{longtable}
}
