# Supplementary material for: KolTa: A Physics-Informed Active Learning Framework for Formulation Discovery with Limited Data
Source: arXiv:2611.06394 source file (2026-11-06)
Supplement: Supplementary file 9 [file calibration.tex]

{\small\renewcommand{\arraystretch}{1.12}
\begin{longtable}{@{}lrrrrrrr@{}}
\caption{Calibrated margin coefficients of \method{} in the ten acquisition rounds of the three runs on each task. Counts give the rounds with a positive coefficient. Medians are taken over all rounds in the RMS-scaled coordinates $c'_u=c_u\sigma_u$ and $c'_v=c_v\sigma_v$ of Section~\ref{sec:protocol}.}\label{tab:scalib}\\
\toprule
Task & Rounds & $c_u>0$ & $c_v>0$ & Both $>0$ & Both $=0$ & Median $c'_u$ & Median $c'_v$\\
\midrule
\endfirsthead
\multicolumn{8}{c}{\tablename~\thetable\ (continued)}\\
\toprule
Task & Rounds & $c_u>0$ & $c_v>0$ & Both $>0$ & Both $=0$ & Median $c'_u$ & Median $c'_v$\\
\midrule
\endhead
\bottomrule
\endlastfoot
NIST & 30 & 30 & 29 & 29 & 0 & 0.071 & 0.025 \\
Drug & 30 & 30 & 29 & 29 & 0 & 0.235 & 0.038 \\
ILThermo & 30 & 30 & 30 & 30 & 0 & 0.122 & 0.052 \\
DiffMix & 30 & 30 & 27 & 27 & 0 & 0.037 & 0.008 \\
\end{longtable}
}
