# Supplementary material for: KolTa: A Physics-Informed Active Learning Framework for Formulation Discovery with Limited Data
Source: arXiv:2611.06394 source file (2026-11-06)
Supplement: Supplementary file 10 [file consistency.tex]

% Generated values retained; keep both panels and their headers on one page.
\par\addvspace{6pt}
\noindent\begin{minipage}{\linewidth}
\centering
\small\setlength{\tabcolsep}{5pt}\renewcommand{\arraystretch}{1.15}
\captionof{table}{Cross-task consistency summaries. (a) Each task cell lists AULC ranks for seeds 0, 1, and 2 among the nine model-based strategies; 1 is best. The top-three count is out of nine runs. The maximum gap uses the best mean AULC on each of the three measured tasks. (b) Mean AULCs and maximum gaps for the three acquisition variants across Drug and ILThermo, using the best of these variants on each task. Gaps are calculated before rounding; smaller gaps are better.}\label{tab:sconsistency}
\begin{tabular}{@{}lccccr@{}}
\toprule
\multicolumn{6}{l}{\textbf{(a) Model-based strategies}}\\*
Strategy & NIST & Drug & ILThermo & Top-three runs & Max. gap\\*
\midrule
\method{} (ours) & $2,\,3,\,2$ & $1,\,1,\,1$ & $1,\,2,\,1$ & \textbf{9/9} & \textbf{0.032} \\
SolvGNN-Greedy & $3,\,2,\,3$ & $3,\,2,\,4$ & $2,\,6,\,3$ & 7/9 & 0.056 \\
MolSets-Greedy & $4,\,6,\,4$ & $6,\,3,\,6$ & $8,\,5,\,4$ & 1/9 & 0.079 \\
GP-Greedy & $1,\,1,\,1$ & $4,\,6,\,7$ & $5,\,1,\,2$ & 5/9 & 0.086 \\
SolvGNN-UCB & $7,\,7,\,6$ & $2,\,4,\,3$ & $3,\,8,\,6$ & 3/9 & 0.096 \\
XGBoost-Greedy & $6,\,4,\,7$ & $9,\,5,\,8$ & $6,\,7,\,7$ & 0/9 & 0.108 \\
XGBoost-UCB & $5,\,5,\,5$ & $8,\,9,\,9$ & $7,\,3,\,8$ & 1/9 & 0.149 \\
MolSets-UCB & $8,\,8,\,8$ & $5,\,8,\,5$ & $4,\,4,\,5$ & 0/9 & 0.167 \\
GP-EI & $9,\,9,\,9$ & $7,\,7,\,2$ & $9,\,9,\,9$ & 1/9 & 0.535 \\
\midrule
\multicolumn{6}{l}{\textbf{(b) Acquisition variants}}\\*
Variant & \multicolumn{2}{c}{Drug mean AULC} & \multicolumn{2}{c}{ILThermo mean AULC} & Max. gap\\*
\midrule
\method{} (ours; PRC-UCB) & \multicolumn{2}{c}{\textbf{0.7384}} & \multicolumn{2}{c}{0.7479} & \textbf{0.015} \\
A1: $u$-only margin & \multicolumn{2}{c}{0.7294} & \multicolumn{2}{c}{0.7359} & 0.027 \\
A2: greedy & \multicolumn{2}{c}{0.7120} & \multicolumn{2}{c}{\textbf{0.7630}} & 0.026 \\
\bottomrule
\end{tabular}
\end{minipage}
\par\addvspace{6pt}
