# Supplementary material for: KolTa: A Physics-Informed Active Learning Framework for Formulation Discovery with Limited Data
Source: arXiv:2611.06394 source file (2026-11-06)
Supplement: Supplementary file 11 [file mae.tex]

{\small\renewcommand{\arraystretch}{1.12}
\begin{longtable}{@{}lrrrrrrr@{}}
\caption{Final target-temperature mean absolute error (MAE) on the locked sets, in base-10 logarithmic target units. Lower MAE is better. The last columns compare ranks by mean MAE and mean discovery AULC within each task (1 is best). SD is the sample standard deviation.}\label{tab:smae}\\
\toprule
Strategy & Seed 0 & Seed 1 & Seed 2 & Mean & SD & MAE rank & AULC rank \\
\midrule
\endfirsthead
\multicolumn{8}{c}{\tablename~\thetable\ (continued)}\\
\toprule
Strategy & Seed 0 & Seed 1 & Seed 2 & Mean & SD & MAE rank & AULC rank \\
\midrule
\endhead
\midrule
\multicolumn{8}{r}{Continued on next page}\\
\endfoot
\bottomrule
\endlastfoot
\multicolumn{8}{l}{\textbf{NIST}}\\
\method{} (ours) & 0.1217 & 0.1066 & 0.0956 & 0.1079 & 0.0131 & 3 & 2 \\
MolSets-UCB & 0.1362 & 0.1072 & 0.1255 & 0.1230 & 0.0147 & 4 & 8 \\
MolSets-Greedy & 0.1497 & 0.1745 & 0.1242 & 0.1495 & 0.0252 & 7 & 4 \\
SolvGNN-UCB & 0.1364 & 0.1320 & 0.1186 & 0.1290 & 0.0093 & 5 & 7 \\
SolvGNN-Greedy & 0.1438 & 0.1389 & 0.1283 & 0.1370 & 0.0079 & 6 & 3 \\
GP-EI & 0.0622 & 0.0784 & 0.0602 & 0.0669 & 0.0100 & 1 & 9 \\
GP-Greedy & 0.1035 & 0.1157 & 0.0976 & 0.1056 & 0.0092 & 2 & 1 \\
XGBoost-UCB & 0.1770 & 0.1724 & 0.1565 & 0.1686 & 0.0107 & 8 & 6 \\
XGBoost-Greedy & 0.1922 & 0.1668 & 0.1552 & 0.1714 & 0.0189 & 9 & 5 \\
\addlinespace[4pt]
\multicolumn{8}{l}{\textbf{Drug}}\\
\method{} (ours) & 0.1771 & 0.1678 & 0.1746 & 0.1731 & 0.0048 & 1 & 1 \\
MolSets-UCB & 0.2053 & 0.2138 & 0.2143 & 0.2111 & 0.0050 & 5 & 7 \\
MolSets-Greedy & 0.2331 & 0.2304 & 0.2480 & 0.2372 & 0.0095 & 7 & 5 \\
SolvGNN-UCB & 0.1772 & 0.1766 & 0.1995 & 0.1844 & 0.0131 & 2 & 2 \\
SolvGNN-Greedy & 0.1943 & 0.1903 & 0.2034 & 0.1960 & 0.0067 & 3 & 3 \\
GP-EI & 0.2291 & 0.2038 & 0.1568 & 0.1965 & 0.0367 & 4 & 4 \\
GP-Greedy & 0.2087 & 0.2787 & 0.1954 & 0.2276 & 0.0448 & 6 & 6 \\
XGBoost-UCB & 0.3414 & 0.3429 & 0.3466 & 0.3436 & 0.0027 & 8 & 9 \\
XGBoost-Greedy & 0.3366 & 0.3448 & 0.3560 & 0.3458 & 0.0097 & 9 & 8 \\
\addlinespace[4pt]
\multicolumn{8}{l}{\textbf{ILThermo}}\\
\method{} (ours) & 0.1392 & 0.1234 & 0.1397 & 0.1341 & 0.0093 & 2 & 1 \\
MolSets-UCB & 0.1880 & 0.1474 & 0.1954 & 0.1769 & 0.0258 & 6 & 4 \\
MolSets-Greedy & 0.1870 & 0.1545 & 0.1764 & 0.1726 & 0.0165 & 5 & 5 \\
SolvGNN-UCB & 0.1562 & 0.1427 & 0.1596 & 0.1529 & 0.0089 & 3 & 6 \\
SolvGNN-Greedy & 0.1678 & 0.1524 & 0.1739 & 0.1647 & 0.0111 & 4 & 3 \\
GP-EI & 0.0743 & 0.0750 & 0.0850 & 0.0781 & 0.0060 & 1 & 9 \\
GP-Greedy & 0.2086 & 0.1635 & 0.1861 & 0.1861 & 0.0225 & 7 & 2 \\
XGBoost-UCB & 0.2036 & 0.2058 & 0.1950 & 0.2015 & 0.0057 & 8 & 7 \\
XGBoost-Greedy & 0.2070 & 0.2115 & 0.2124 & 0.2103 & 0.0029 & 9 & 8 \\
\addlinespace[4pt]
\multicolumn{8}{l}{\textbf{DiffMix}}\\
\method{} (ours) & 0.0525 & 0.0457 & 0.0559 & 0.0514 & 0.0052 & 3 & 2 \\
MolSets-UCB & 0.1287 & 0.0733 & 0.0880 & 0.0967 & 0.0287 & 6 & 6 \\
SolvGNN-UCB & 0.0486 & 0.0644 & 0.0324 & 0.0485 & 0.0160 & 2 & 3 \\
GP-EI & 0.0359 & 0.0387 & 0.0318 & 0.0354 & 0.0035 & 1 & 5 \\
XGBoost-UCB & 0.0681 & 0.0710 & 0.0728 & 0.0706 & 0.0023 & 4 & 4 \\
XGBoost-Greedy & 0.0678 & 0.0699 & 0.0786 & 0.0721 & 0.0057 & 5 & 1 \\
\end{longtable}
}
