# Supplementary material for: KolTa: A Physics-Informed Active Learning Framework for Formulation Discovery with Limited Data
Source: arXiv:2611.06394 source file (2026-11-06)
Supplement: Supplementary file 12 [file queries.tex]

{\small\renewcommand{\arraystretch}{1.12}
\begin{longtable}{@{}lrrrrrr@{}}
\caption{New queries needed to reach 30\% and 80\% active recall in each run, estimated by linear interpolation. A dash means the level was not reached within the budget. These estimates can be fractional because queries are evaluated in batches.}\label{tab:squeries}\\
\toprule
& \multicolumn{3}{c}{$q_{30}$} & \multicolumn{3}{c}{$q_{80}$}\\
\cmidrule(lr){2-4}\cmidrule(l){5-7}
Strategy & Seed 0 & Seed 1 & Seed 2 & Seed 0 & Seed 1 & Seed 2 \\
\midrule
\endfirsthead
\multicolumn{7}{c}{\tablename~\thetable\ (continued)}\\
\toprule
& \multicolumn{3}{c}{$q_{30}$} & \multicolumn{3}{c}{$q_{80}$}\\
\cmidrule(lr){2-4}\cmidrule(l){5-7}
Strategy & Seed 0 & Seed 1 & Seed 2 & Seed 0 & Seed 1 & Seed 2 \\
\midrule
\endhead
\midrule
\multicolumn{7}{r}{Continued on next page}\\
\endfoot
\bottomrule
\endlastfoot
\multicolumn{7}{l}{\textbf{NIST}}\\
\method{} (ours) & 266.9 & 270.4 & 249.4 & --- & 772.2 & --- \\
MolSets-UCB & 397.6 & 369.7 & 391.9 & --- & --- & --- \\
MolSets-Greedy & 266.2 & 303.3 & 287.5 & --- & --- & --- \\
SolvGNN-UCB & 314.0 & 287.4 & 294.1 & --- & --- & --- \\
SolvGNN-Greedy & 283.2 & 248.1 & 255.0 & --- & --- & --- \\
GP-EI & --- & --- & --- & --- & --- & --- \\
GP-Greedy & 237.0 & 232.6 & 231.0 & 689.0 & 674.6 & 798.6 \\
XGBoost-UCB & 239.2 & 308.6 & 296.0 & --- & --- & --- \\
XGBoost-Greedy & 262.1 & 274.1 & 296.3 & --- & --- & --- \\
Random & --- & --- & --- & --- & --- & --- \\
\addlinespace[4pt]
\multicolumn{7}{l}{\textbf{Drug}}\\
\method{} (ours) & 94.0 & 84.1 & 78.5 & 310.3 & 348.0 & 353.1 \\
MolSets-UCB & 121.1 & 111.9 & 112.9 & 445.9 & 504.2 & 430.1 \\
MolSets-Greedy & 105.4 & 89.2 & 105.7 & 489.1 & 475.2 & 486.3 \\
SolvGNN-UCB & 99.6 & 120.8 & 77.8 & 427.8 & 424.4 & 408.6 \\
SolvGNN-Greedy & 102.9 & 97.3 & 102.5 & 457.0 & 436.1 & 422.2 \\
GP-EI & 120.6 & 116.0 & 89.3 & 472.6 & 498.7 & 365.4 \\
GP-Greedy & 104.6 & 119.6 & 111.1 & 483.4 & 455.1 & 509.4 \\
XGBoost-UCB & 118.3 & 138.5 & 125.0 & 564.0 & 574.9 & 635.4 \\
XGBoost-Greedy & 113.1 & 82.9 & 121.9 & 627.2 & 513.0 & 569.3 \\
Random & 464.3 & 602.8 & 452.6 & --- & --- & --- \\
\addlinespace[4pt]
\multicolumn{7}{l}{\textbf{ILThermo}}\\
\method{} (ours) & 39.1 & 37.8 & 41.6 & 112.0 & 114.5 & 103.2 \\
MolSets-UCB & 38.7 & 41.2 & 35.5 & 139.5 & 147.3 & 142.7 \\
MolSets-Greedy & 30.5 & 27.9 & 29.2 & 169.2 & 150.0 & 139.5 \\
SolvGNN-UCB & 54.2 & 60.0 & 42.9 & 134.4 & 170.0 & 133.6 \\
SolvGNN-Greedy & 36.2 & 40.0 & 37.6 & 117.8 & 153.3 & 128.4 \\
GP-EI & 246.0 & --- & --- & --- & --- & --- \\
GP-Greedy & 30.3 & 33.8 & 35.0 & 240.9 & 107.5 & 114.0 \\
XGBoost-UCB & 50.6 & 36.4 & 57.2 & 163.7 & 130.9 & 144.9 \\
XGBoost-Greedy & 58.8 & 42.6 & 31.9 & 161.0 & 195.0 & 154.8 \\
Random & --- & --- & --- & --- & --- & --- \\
\addlinespace[4pt]
\multicolumn{7}{l}{\textbf{DiffMix}}\\
\method{} (ours) & 28.0 & 48.8 & 30.0 & 97.5 & 117.1 & 87.3 \\
MolSets-UCB & 228.6 & 158.9 & 242.9 & 377.1 & 346.7 & 374.5 \\
SolvGNN-UCB & 64.0 & 63.0 & 22.7 & 108.0 & 108.0 & 104.6 \\
GP-EI & 38.2 & 31.2 & 33.6 & 240.0 & --- & 333.3 \\
XGBoost-UCB & 38.2 & 66.3 & 38.2 & 141.2 & 128.9 & 114.7 \\
XGBoost-Greedy & 30.0 & 22.3 & 30.0 & 85.7 & 93.3 & 94.5 \\
Random & --- & 355.0 & --- & --- & --- & --- \\
\end{longtable}
}
