# Supplementary material for: KolTa: A Physics-Informed Active Learning Framework for Formulation Discovery with Limited Data
Source: arXiv:2611.06394 source file (2026-11-06)
Supplement: Supplementary file 13 [file taskstats.tex]

{\small\renewcommand{\arraystretch}{1.12}
\begin{longtable}{@{}lrrrrrrrrr@{}}
\caption{Candidate pools, targets, and budgets. The labeled fraction is the share of the discovery pool labeled at the end of a run. Targets are the top 5\% of the pool by utility at $T^*$, ties included; on Drug they are defined within each drug and summed. Initial hits and remaining targets are given for seeds 0/1/2. Records count all measured temperatures of a pool formulation. Records per formulation are reported as median (range).}\label{tab:stasks}\\
\toprule
Task & Pool & $|\mathcal L_0|$ & $B$ & \shortstack{Labeled\\fraction} & Targets & Initial hits & Remaining & Records per formulation & Components\\
\midrule
\endfirsthead
\multicolumn{10}{c}{\tablename~\thetable\ (continued)}\\
\toprule
Task & Pool & $|\mathcal L_0|$ & $B$ & \shortstack{Labeled\\fraction} & Targets & Initial hits & Remaining & Records per formulation & Components\\
\midrule
\endhead
\bottomrule
\endlastfoot
NIST & 15,575 & 200 & 800 & 6\% & 779 & 15/10/9 & 764/769/770 & 2 (1--31) & 2--2 \\
Drug & 2,159 & 300 & 800 & 51\% & 141 & 22/20/16 & 119/121/125 & 9 (4--15) & 2--3 \\
ILThermo & 1,940 & 150 & 300 & 23\% & 98 & 4/8/7 & 94/90/91 & 7 (1--17) & 2--3 \\
DiffMix & 1,471 & 100 & 400 & 34\% & 74 & 4/9/4 & 70/65/70 & 6 (2--6) & 2--4 \\
\end{longtable}
}
