# Supplementary material for: KolTa: A Physics-Informed Active Learning Framework for Formulation Discovery with Limited Data
Source: arXiv:2611.06394 source file (2026-11-06)
Supplement: Supplementary file 14 [file tests.tex]

{\small\renewcommand{\arraystretch}{1.12}
\begin{longtable}{@{}lrrlrrrr@{}}
\caption{Paired comparisons of full-budget AULC: KolTa minus each comparator. Wins count strictly positive differences. The one-sided exact sign and Wilcoxon signed-rank tests are each Holm-adjusted across the eight comparisons.}\label{tab:stests}\\
\toprule
Comparator & Wins & Median & Range & $p_{\rm sign}$ & $p_{\rm Wil.}$ & $p_{\rm sign}^{\rm Holm}$ & $p_{\rm Wil.}^{\rm Holm}$ \\
\midrule
\endfirsthead
\multicolumn{8}{c}{\tablename~\thetable\ (continued)}\\
\toprule
Comparator & Wins & Median & Range & $p_{\rm sign}$ & $p_{\rm Wil.}$ & $p_{\rm sign}^{\rm Holm}$ & $p_{\rm Wil.}^{\rm Holm}$ \\
\midrule
\endhead
\midrule
\multicolumn{8}{r}{Continued on next page}\\
\endfoot
\bottomrule
\endlastfoot
MolSets-UCB & 12/12 & +0.1185 & [+0.0289, +0.5579] & 0.00024 & 0.00024 & 0.00195 & 0.00195 \\
MolSets-Greedy & 9/9 & +0.0457 & [+0.0305, +0.0916] & 0.00195 & 0.00195 & 0.00977 & 0.00781 \\
SolvGNN-UCB & 11/12 & +0.0596 & [-0.0043, +0.0922] & 0.00317 & 0.00049 & 0.01270 & 0.00244 \\
SolvGNN-Greedy & 8/9 & +0.0308 & [-0.0163, +0.0740] & 0.01953 & 0.01367 & 0.03906 & 0.02734 \\
GP-EI & 12/12 & +0.2647 & [+0.0181, +0.5783] & 0.00024 & 0.00024 & 0.00195 & 0.00195 \\
GP-Greedy & 5/9 & +0.0126 & [-0.0494, +0.0871] & 0.50000 & 0.17969 & 0.50000 & 0.17969 \\
XGBoost-UCB & 12/12 & +0.0622 & [+0.0039, +0.1679] & 0.00024 & 0.00024 & 0.00195 & 0.00195 \\
XGBoost-Greedy & 11/12 & +0.0697 & [-0.0462, +0.1405] & 0.00317 & 0.00244 & 0.01270 & 0.00781 \\
\end{longtable}
}
